# Supplementary material for: Large change of interlayer vibrational coupling with stacking in Mo$_{1-x}$W$_{x}$Te$_{2}$
Source: arXiv:2110.10844 source file (2021-10-21)
Supplement: Supplementary file 1 [file supplement.pdf]

# Supplemental Materials: Large change of interlayer vibrational coupling with stacking in $Mo_{1-x}W_xTe_2$

John A. Schneeloch,[1] Yu Tao,[1] Jaime A. Fernandez-Baca,[2,*] Guangyong Xu,[3] and Despina Louca[1,†]

[1] *Department of Physics, University of Virginia, Charlottesville, Virginia 22904, USA*
[2] *Neutron Scattering Division, Oak Ridge National Laboratory, Oak Ridge, Tennessee 37831, USA*
[3] *NIST Center for Neutron Research, National Institute of Standards and Technology, Gaithersburg, Maryland 20877, USA*

## ADDITIONAL INELASTIC SCANS

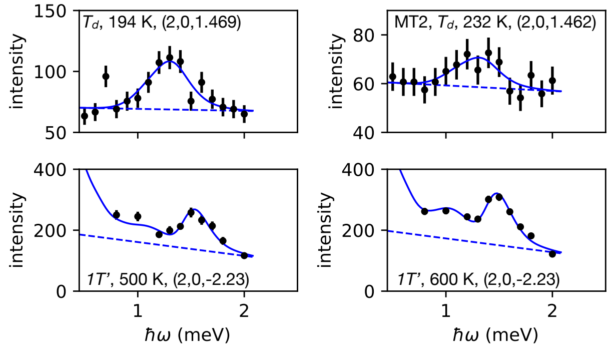


FIG. S1. Scans of inelastic neutron scattering intensity.

In Fig. S1, we show data taken in the $T_d$ phase at 194 K (at the same point in reciprocal space as the 272 K data in Fig. 3(a) of the main text), in the $1T'$ phase at 500 and 600 K, and on a separate sample MT2 (with composition $Mo_{1-x}W_xTe_2$ with $x \leq 0.01$) in its $T_d$ phase. The results from fitting are shown in Table II in the main text.

## DETAILS OF FITTING INELASTIC DATA

$S(\mathbf{Q}, \omega)$ was calculated and convoluted with the resolution function for the CTAX or SPINS instruments. (See below for discussion of the phonon dispersion.) This calculation was done in the python package NeutronPy [1], which includes a translation to python of the MATLAB package ResLib [2]. The Cooper-Nathans method was used [3].

To estimate the sample mosaic and twin fractions, we referred to elastic scans taken along $(2, 0, L)$ just before or after the inelastic scans shown in Fig. 3 in the main text. For the sample mosaic, preliminary calculations showed that the main effect of modifying the sample mosaic on calculated Bragg peak intensities along the relevant $(2, 0, L)$ regions was a linear decrease in peak height on moving along either $+L$ or $-L$ away from $L = 0$; changes in peak width were minor. The decrease was estimated from the deviation of the $T_d$ peak heights in Fig. S2 from the expected squared structure factor dependence, and was consistent with a mosaic angle of about 100'. After determining the mosaic-related decrease in peak height with increasing $|L|$, we adjusted the $T_d^*$ and $1T'$ twin fractions, finding satisfactory agreement for ∼25% and ∼65% of the $1T'$ BA twin for the CTAX and SPINS data, respectively, and ∼70% of the $T_d^*$ AABB twin for the SPINS data.

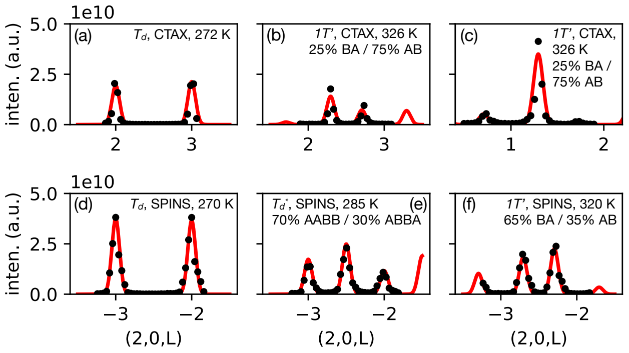


FIG. S2. Elastic neutron scattering scans along $(2, 0, L)$. Error bars are smaller than the symbols. The red curves are Gaussian functions multiplied by the squared structure factor as calculated for each phase, adjusted to the $T_d$ data in (a) and (d) (i.e., with the overall intensity and mosaic-related linear $L$-dependence of the intensity set by these $T_d$ data), then with the $T_d^*$ or $1T'$ twin fractions varied until an acceptable agreement was reached.

To define the background in Fig. 3 of the main text, we first fit a linear background to data sets 3(a) (for CTAX) and 3(g) (for SPINS), keeping the overall intensity as determined from previous fits of 3(a) and 3(e). For each of the remaining scans for each instrument, we adjusted the background for 3(a) and 3(g) by $Q^2$ (i.e., we assumed the background was phonon-related). For 3(d), to better fit the data, we allowed the constant part of the background

---

* Notice: This manuscript has been authored by UT-Battelle, LLC, under contract DE-AC05-00OR22725 with the US Department of Energy (DOE). The US government retains and the publisher, by accepting the article for publication, acknowledges that the US government retains a nonexclusive, paid-up, irrevocable, worldwide license to publish or reproduce the published form of this manuscript, or allow others to do so, for US government purposes. DOE will provide public access to these results of federally sponsored research in accordance with the DOE Public Access Plan (http://energy.gov/downloads/doe-public-access-plan).

† Corresponding author; louca@virginia.edu

TABLE S1. $K_x$ values (in $10^{19}$ N/m$^3$) averaged within each phase and $K_x$ ratios for fits assuming various sample mosaics.

| mosaic | $K_x^{T_d}$ | $K_x^{T_d^*}$ | $K_x^{1T'}$ | $K_x^{T_d^*}/K_x^{T_d}$ | $K_x^{1T'}/K_x^{T_d}$ |
|---|---|---|---|---|---|
| 50’ | 0.921(22) | 0.682(18) | 0.757(17) | 74.0(2.6)% | 82.2(2.7)% |
| 100’ | 0.919(24) | 0.694(25) | 0.760(24) | 76(3)% | 83(3)% |
| 150’ | 0.946(28) | 0.70(4) | 0.77(5) | 74(5)% | 81(6)% |

to vary in subsequent fitting. For the additional data in Fig. S1, for the $T_d$ data, the background was allowed to vary freely, and for the $1T'$ data, the background could vary by an overall constant, keeping the slope fixed to minimize its influence on the fitted peak position (and because the data do not unambiguously indicate a background as they do for the $T_d$ data.)

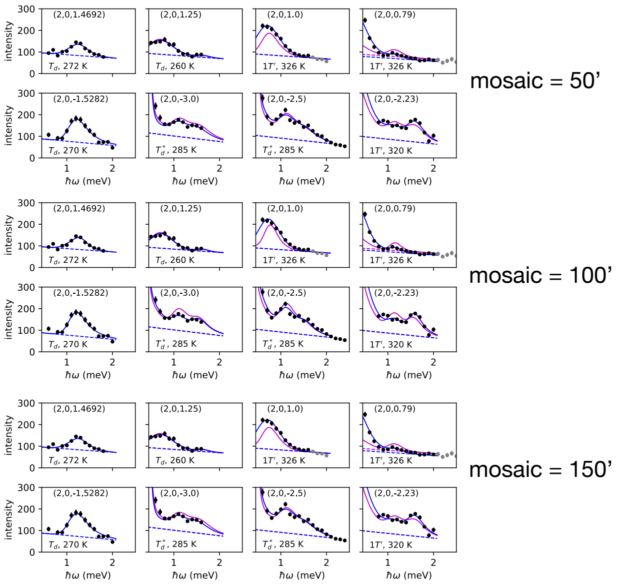


FIG. S3. Data and calculated resolution-convoluted $S(\mathbf{Q}, \omega)$, assuming various values of the sample mosaic. Details are the same as for Fig. 3 of the main text.

Although we can get an estimate of the sample mosaic from the elastic data, for completeness we show the effect of sample mosaic on the fitting in Fig. S3. The details of the plots are the same as for Fig. 3 of the main text except that calculations for sample mosaics of 50’ and 150’ are shown in addition to 100’. A wider sample mosaic results in broader inelastic features. However, the ratios of the $K_x$ values show little change, as seen in Table S1.

## PHONON DISPERSION PERPENDICULAR TO $(2, 0, L)$

For the resolution convolution, we needed to account for the ISM dispersion perpendicular to the $(2, 0, L)$ line.

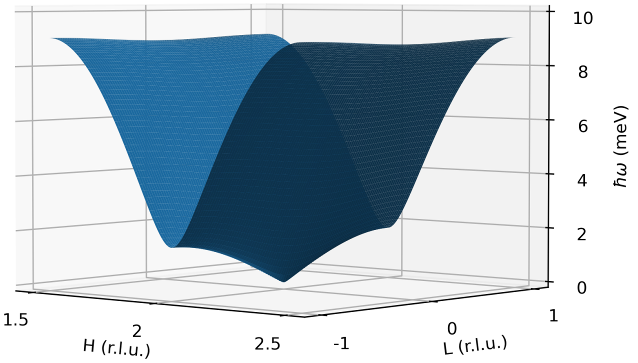


FIG. S4. Depiction of the ISM dispersion in the $(H, 0, L)$ plane, used for resolution convolution.

TABLE S2. $K_x$ values (in $10^{19}$ N/m$^3$) averaged within each phase and $K_x$ ratios for fits assuming various multiplying factors for the dispersion perpendicular to the $(2, 0, L)$ line.

| mult. | $K_x^{T_d}$ | $K_x^{T_d^*}$ | $K_x^{1T'}$ | $K_x^{T_d^*}/K_x^{T_d}$ | $K_x^{1T'}/K_x^{T_d}$ |
|---|---|---|---|---|---|
| ×0.5 | 1.062(29) | 0.734(25) | 0.845(18) | 69(3)% | 79.5(2.8)% |
| ×1 | 0.919(24) | 0.694(25) | 0.760(24) | 76(3)% | 83(3)% |
| ×2 | 0.821(27) | 0.67(4) | 0.68(5) | 81(6)% | 83(6)% |

Though the assumed perpendicular dispersion is a source of systematic error in obtaining the dispersion maximum $\hbar\omega_m$, we will show that the relative differences in $\hbar\omega_m$ between the phases is roughly constant regardless of the details of the perpendicular dispersion.

If we assume a 3-dimensional rectangular grid of atoms which only vibrate along the $a$-axis (as they should for small deviations away from the ISM on $(2, 0, L)$), then we can assume that there are three types of spring constants between neighboring atoms: $k_z$ for the interlayer shear mode, $k_x$ for the longitudinal mode along the $a$-axis, and $k_y$ for the in-plane shear mode. The resulting dispersion is given by

$$(\hbar\omega)^2 = 2k_H(1 - \cos(2\pi H)) + 2k_K(1 - \cos(2\pi K)) + 2k_L(1 - \cos(\pi L)) \quad (1)$$

Along the $L$ direction, the spring constant $k_L = (\hbar\omega_m)^2/4$ (e.g., $\sim$0.73 meV$^2$ for $\hbar\omega_m = 1.7$ meV.) The other two spring constants $k_H$ and $k_K$ can be obtained from the calculated $T_d$-$MoTe_2$ elastic constants $C_{11} = 142.3$ GPa and $C_{66} = 62.3$ GPa [4]. (We state the $C_{ij}$ in terms of a coordinate system where $a \sim 6.31$ Å and $b \sim 3.47$ Å.) Though calculations of ISM-related values such as $\hbar\omega_m$ and $C_{55}$ have shown wide discrepancies with experiment, we expect the elastic constants corresponding to the *intralayer* interactions to be more reliable. We note, though, that a calculation in a separate study reports values of $C_{11} = 154.9$ GPa and $C_{66} = 51.9$ GPa [5], which suggests an uncertainty in the calculated elas-

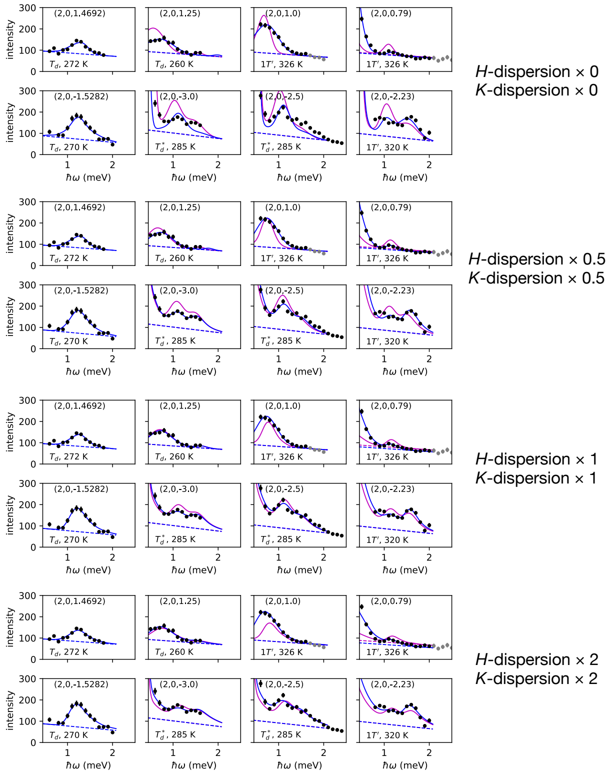


FIG. S5. Data and calculated resolution-convoluted $S(\mathbf{Q}, \omega)$, assuming various values of the perpendicular dispersion coefficients (expressed as a multiplier times values obtained from computed elastic constants [4].) Details are the same as for Fig. 3 of the main text.

TABLE S3. Values of $\hbar\omega_m$ obtained from fits of the data in Fig. 3(a), assuming various multiplier factors for the dispersion perpendicular to the $(2, 0, L)$ line. Additionally, the equivalent $\hbar\omega_m$ value from a Gaussian fit of the peak position is listed.

| | fitted $\hbar\omega$ (meV) for data set (a) |
|---|---|
| $\times 0$ | 1.85(3) |
| $\times 0.5$ | 1.76(3) |
| $\times 1$ | 1.71(3) |
| $\times 2$ | 1.63(4) |
| gaussian fit | 1.67(3) |

tic constants on the order of ~8 to 20%. Regardless, we can get the spring constants in our model from the expressions $v = \sqrt{C/\rho}$ (where $C$ is the relevant elastic constant and $\rho$ is the density) and $v = \frac{d\omega}{dk}$ taken near the Bragg peak, yielding $k_H = \frac{1}{a^2}\frac{C_{22}}{\rho}$ and $k_K = \frac{1}{b^2}\frac{C_{66}}{\rho}$. The dispersion in the $(H0L)$ plane is shown in Fig. S4.

We show the dependence of the perpendicular dispersion stiffness on the fitting in Fig. S5. As for Fig. 3 in the main text, the resolution-convoluted $S(\mathbf{Q}, \omega)$ is plotted over the data points, both for the intensity predicted by the LCM (magenta) and after fitting while allowing values of the intensity, twin fraction, and $\omega_m$ to relax (blue). The fitting was repeated for different multipliers of the perpendicular dispersion stiffness. Not all multipliers result in acceptable fits, but the averaged $K_x$ values obtained from these fits for multipliers of $\times 0.5$, $\times 1$, and $\times 2$ are shown in Table S2. Although the obtained $K_x$ decrease as the assumed perpendicular slope increases, the $K_x^{T_d^*}$ and $K_x^{1T'}$ interlayer force constants are consistently on the order of 80% that of $T_d$, suggesting that reasonable deviations of the true perpendicular dispersion stiffness from values estimated from calculated elastic constants should not change our results. The potential for systematic error is demonstrated in Table S3, in which the obtained $\hbar\omega_m$ from the fit to the data in Fig. 3(a) decreases as the assumed perpendicular slope increases.

## LINEAR CHAIN MODEL WITH TWO SPRING CONSTANTS FOR THE $T_d^*$ PHASE

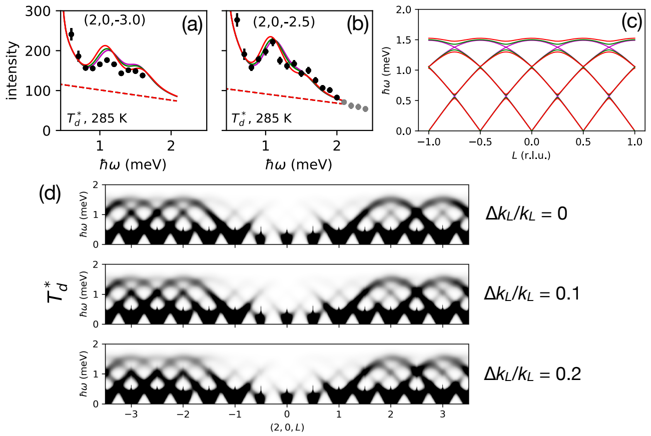


FIG. S6. Depicted spectra and intensities for a two-spring-constant linear chain model suitable for $T_d^*$. (a,b) Calculated intensities from LCM model for two spring constants $k_L^1 = k_L \times (1 + \frac{\Delta k_L}{k_L})$ and $k_L^2 = k_L/(1 + \frac{\Delta k_L}{k_L})$, with $\frac{\Delta k_L}{k_L} = 0$, 0.1, and 0.2 for the magenta, green, and red curves, respectively. (a) and (b) correspond, respectively, to Fig. 3(f) and 3(g) in the main text. (c) Computed dispersion for the values of $\frac{\Delta k_L}{k_L}$ used for (a) and (b). (d) Computed INS intensity for these $\frac{\Delta k_L}{k_L}$ values.

Generally, our analysis assumes that the phonon energies and INS intensities for $T_d$, $T_d^*$, and $1T'$ can be described by the linear chain model with a single spring constant $k_L = (\hbar\omega_m)^2/4$ between neighbors. However, by symmetry, *two* spring constants are allowed for $T_d^*$, which we call $k_L^1$ and $k_L^2$. In this section, we discuss why our results (and the implied shear elastic constant $C_{55}$) depend primarily on the average $k_L = \sqrt{k_L^1 k_L^2}$, so that

even the reasonable assumption of a ∼20% difference between $k_L^1$ and $k_L^2$ wouldn't yield noticeably different results from those of a single spring constant $k_L$.

The symmetries of $T_d$ and $1T'$ allow only a single LCM spring constant between neighboring layers, but the inversion symmetry of $T_d^*$ [6] only constrains the number of spring constants to two, in the repeating pattern ...-$k_L^1$-$k_L^1$-$k_L^2$-$k_L^2$-.... From the difference in values of $K_x$ for $T_d$ and $1T'$, it is reasonable to assume the two $T_d^*$ spring constants could differ by ∼20%. We define the spring constants $k_L^1 = k_L \times (1 + \frac{\Delta k_L}{k_L})$ and $k_L^2 = k_L/(1 + \frac{\Delta k_L}{k_L})$, which have a geometric mean of $\sqrt{k_L^1 k_L^2} = k_L$. Fig. S6(a,b) show the calculated intensities corresponding to the data sets in Fig. 3(f) and 3(g) in the main text, for values of $\frac{\Delta k_L}{k_L} = 0$, 0.1, and 0.2. Even for $\frac{\Delta k_L}{k_L} = 0.2$ (i.e., two spring constants separated by ∼37%), little difference is seen relative to the intensity for a single LCM spring constant $k_L$. Figures S6(c) and (d) shows the calculated dispersion and intensities for $\frac{\Delta k_L}{k_L} = 0$, 0.1, and 0.2. Little change is seen in the dispersion, especially at the $L$ values relevant to our data (which correspond to half-integer $L$ in the dispersion shown in Fig. S6(c).) The intensities, too, show only a subtle difference. We note that the slope of the dispersion near half-integer $L$ is largely unchanged by varying $\frac{\Delta k_L}{k_L}$, showing that the mean value $k_L$ is representative of the sound velocity and the $C_{55}$ elastic constant.

## INTERLAYER BREATHING MODE

The ISM is just one of the phonon branches accessible at low energies along $(2, 0, L)$. While the shear mode polarized along the $b$-axis should have zero intensity along $(2, 0, L)$ due to the $\mathbf{Q} \cdot \xi$ selection rule, the interlayer breathing mode (IBM), i.e., the longitudinal acoustic mode in which layers oscillate along the $c$-axis, might be accessible. In this section, we show that the intensity of this mode is likely negligible in the energy range of interest.

Assuming that the IBM follows the linear chain model, we can calculate the dispersion and intensity in the same way as for the ISM. The LCM dispersion can be scaled according to measurements of the longitudinal acoustic velocity along the $c$-axis [7], and the polarization vectors would have the same phase differences between the layers, but would be assumed to oscillate entirely along the $c$-axis. The results are shown in Fig. S7, with CTAX and SPINS measurement locations shown as blue and magenta bars. The calculated intensity map shows that little intensity is expected for the scans' $\mathbf{Q}$ and $\hbar\omega$, except a small amount at the lower-$\hbar\omega$ end of some of the SPINS scans. Thus, the resolution-convoluted calculations in Fig. S7(a-h) show that the intensity is negligible in the energy ranges of interest.


[1] David Fobes, "NeutronPy 2.0.0," (2020).

[2] Andrey Zheludev, "Reslib 3.4c," (2007).

[3] M. J. Cooper and R. Nathans, "The resolution function in neutron diffractometry. I. The resolution function of a neutron diffractometer and its application to phonon measurements," Acta Crystallographica **23**, 357–367 (1967).

[4] B. Rahman Rano, Ishtiaque M. Syed, and S. H. Naqib, "Ab initio approach to the elastic, electronic, and optical properties of $MoTe_2$ topological Weyl semimetal," Journal of Alloys and Compounds **829**, 154522 (2020).

[5] Sobhit Singh, Jinwoong Kim, Karin M. Rabe, and David Vanderbilt, "Engineering Weyl Phases and Nonlinear Hall Effects in $T_d$-$MoTe_2$," Physical Review Letters **125**, 046402 (2020).

[6] Yu Tao, John A. Schneeloch, Chunruo Duan, Masaaki Matsuda, Sachith E. Dissanayake, Adam A. Aczel, Jaime A. Fernandez-Baca, Feng Ye, and Despina Louca, "Appearance of a $T_d^*$ phase across the $T_d$-$1T'$ phase boundary in the Weyl semimetal $MoTe_2$," Physical Review B **100**, 100101 (2019).

[7] Nicolas Rivas, Shazhou Zhong, Tina Dekker, Meixin Cheng, Patrick Gicala, Fangchu Chen, Xuan Luo, Yuping Sun, Ariel A. Petruk, Kostyantyn Pichugin, Adam W. Tsen, and Germán Sciaini, "Generation and detection of coherent longitudinal acoustic waves in ultrathin $1T'$-$MoTe_2$," Applied Physics Letters **115**, 223103 (2019).

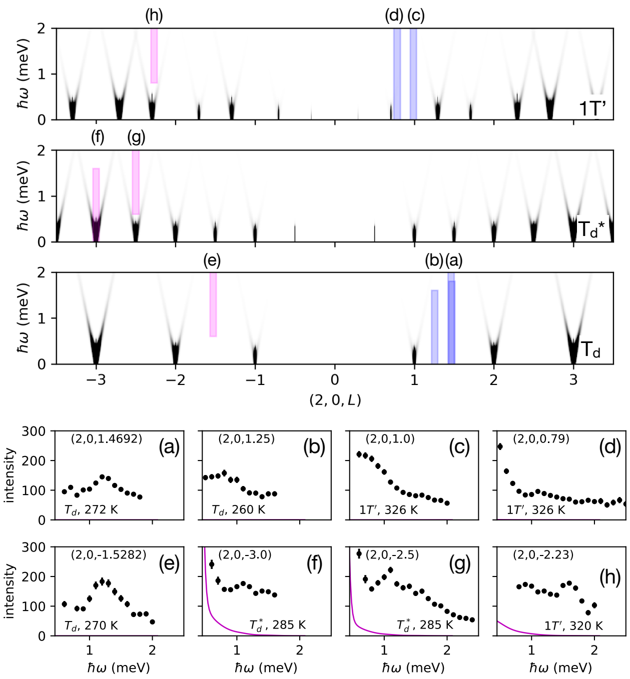


FIG. S7. (top) Calculated intensity map of INS for the interlayer breathing mode from a linear chain model. The intensity scale is the same as for Fig. 2 in the main text. (a-h) Magenta curves show the calculated INS intensity corresponding to the data sets shown in Fig. 3 of the main text. The blue and magenta bars indicate the locations of constant-$\mathbf{Q}$ scans for CTAX and SPINS measurements, respectively.
